# Supplementary material for: Critical Behavior at the Onset of Multichimera States in a Coupled-Oscillator Array
Source: arXiv:1907.07285 ancillary file (2019-07-16)
Supplement: Supplementary file 1 [file paper_kawase1_suppl_arXiv.pdf]

# Supplementary Material: Critical Behavior at the Onset of Multichimera States in a Coupled-Oscillator Array

Katsuya Kawase and Nariya Uchida
*Department of Physics, Tohoku University*

July 16, 2019

## 1 Criteria for ternarization

We ternarized the phase difference to discriminate the (s) synchronous, (w) traveling waves, and (a) asynchronous sites using the criteria

$$(s) \qquad |\Delta\phi_x| \in [0, \Delta_1], \tag{1}$$
$$(w) \qquad |\Delta\phi_x| \in [\Delta_1, \Delta_2], \tag{2}$$
$$(a) \qquad |\Delta\phi_x| \in [\Delta_2, 1]. \tag{3}$$

In the main text, we used $\Delta_1 = 0.10$ and $\Delta_2 = 0.30$. Here we explain the choice of the thresholds $\Delta_1$ and $\Delta_2$ and discuss its effect on the results. In Fig. S1, we show the histogram of the phase difference for $\alpha = 0.44$ and $N = 131072$ oscillators, in the time windows $900 < t < 1000$ and $9000 < t < 10000$. The distributions have a peak at $|\Delta\phi_x| \simeq 0.25$. From the spatio-temporal map of the phase difference (Fig.1), we find that the peak contains most of the traveling wave sites, while the asynchronous clusters with randomly branching structure correspond to larger values of $|\Delta\phi_x|$.

In Fig. S2, the spatio-temporal maps of the ternarized phase difference are compared for the choices $(\Delta_1, \Delta_2) = (0.08, 0.25), (0.10, 0.30), (0.12, 0.35)$. Any of these choices give the characteristic structures in the asynchronous and traveling waves states. The value of $\Delta_2$ is limited by the condition that the peaks of the wave profiles (as shown in Fig.1(d)) are located below $\Delta_2$. On the other hand, the threshold $\Delta_1$ is set between the peaks and valleys of the wave profiles, so that we

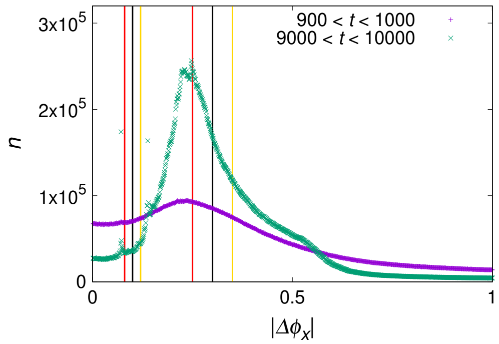


Figure S1: Histogram of the phase difference $|\Delta\phi_x|$. The lines indicate the values of $(\Delta_1, \Delta_2) = (0.08, 0.25)$ (red), $(0.10, 0.30)$ (black), and $(0.12, 0.35)$ (yellow).

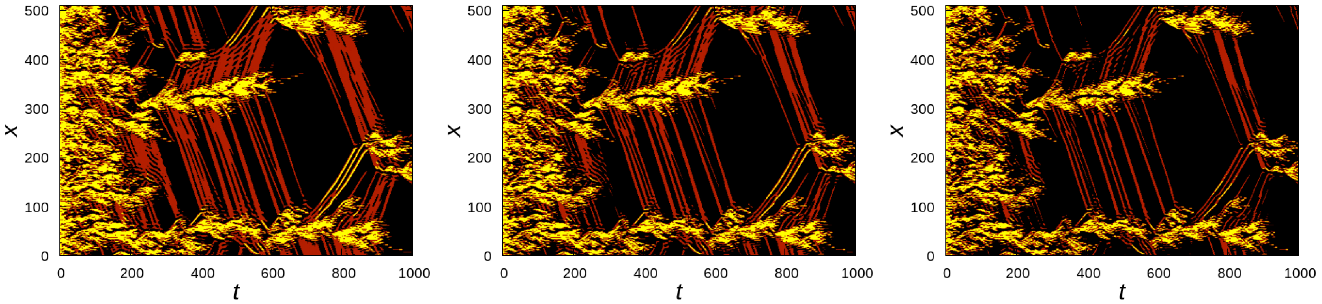


Figure S2: Spatio-temporal maps of the ternarized phase difference for $\alpha = 0.44$. (a) $\Delta_1 = 0.08$ , $\Delta_2 = 0.25$. (b) $\Delta_1 = 0.10$ , $\Delta_2 = 0.30$. (c) $\Delta_1 = 0.12$ , $\Delta_2 = 0.35$. The colors correspond to the synchronous (black), traveling waves (red) and asynchronous (yellow) sites.

can see the wave structure in the spatio-temporal maps. In order to determine the threshold, we use the correlation function $Q_w(x,t)$, shown in Fig.S3 for different choices of $\Delta_1$. We find that the moving peaks that characterize the traveling waves are prominent for $0.08 \leq \Delta_1 \leq 0.12$. Therefore we chose the middle point of this range ($\Delta_1 = 0.10$) as the standard parameter.

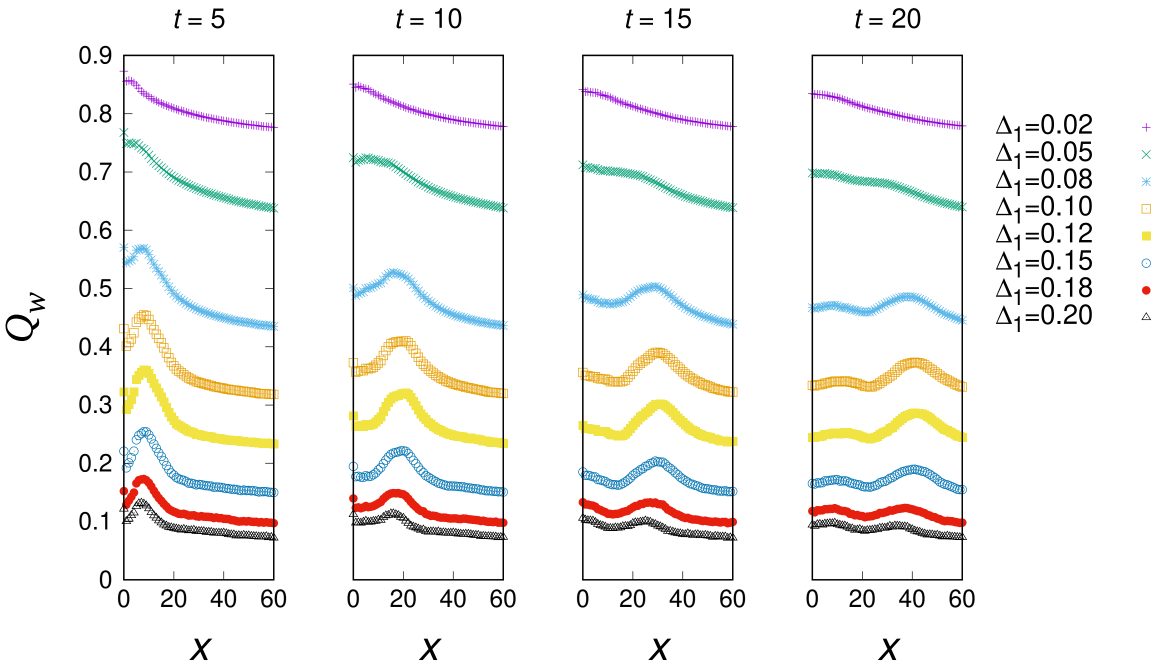


Figure S3: Correlation function for the traveling waves state $Q_w(x,t)$ for different values of $\Delta_1$, with $\Delta_2 = 0.30$ fixed. Cross sections at $t = 5, 10, 15, 20$ from the left to right.

As a further test of the choice of $\Delta_1$ and $\Delta_2$, we measured the spatio-temporal gaps between asynchronous sites ($\xi_{\perp a}$, $\xi_{\parallel a}$) and those between traveling waves sites ($\xi_{\perp w}$, $\xi_{\parallel w}$). In Fig. S4, we plot the histograms of the spatio-temporal gaps for $(\Delta_1, \Delta_2) = (0.08, 0.25), (0.10, 0.30), (0.12, 0.35)$, which are the same values used in Fig.S2. The distributions of the spatial gaps nicely collapse on

a single curve for $10 < \xi_\perp < 5 \times 10^3$, while the distributions of the temporal gaps agree in the range $5 < \xi_\| < 100$, for both the asynchronous and traveling wave states. Thus we confirmed that the results of our calculations do not depend sensitively on the ternarization thresholds.

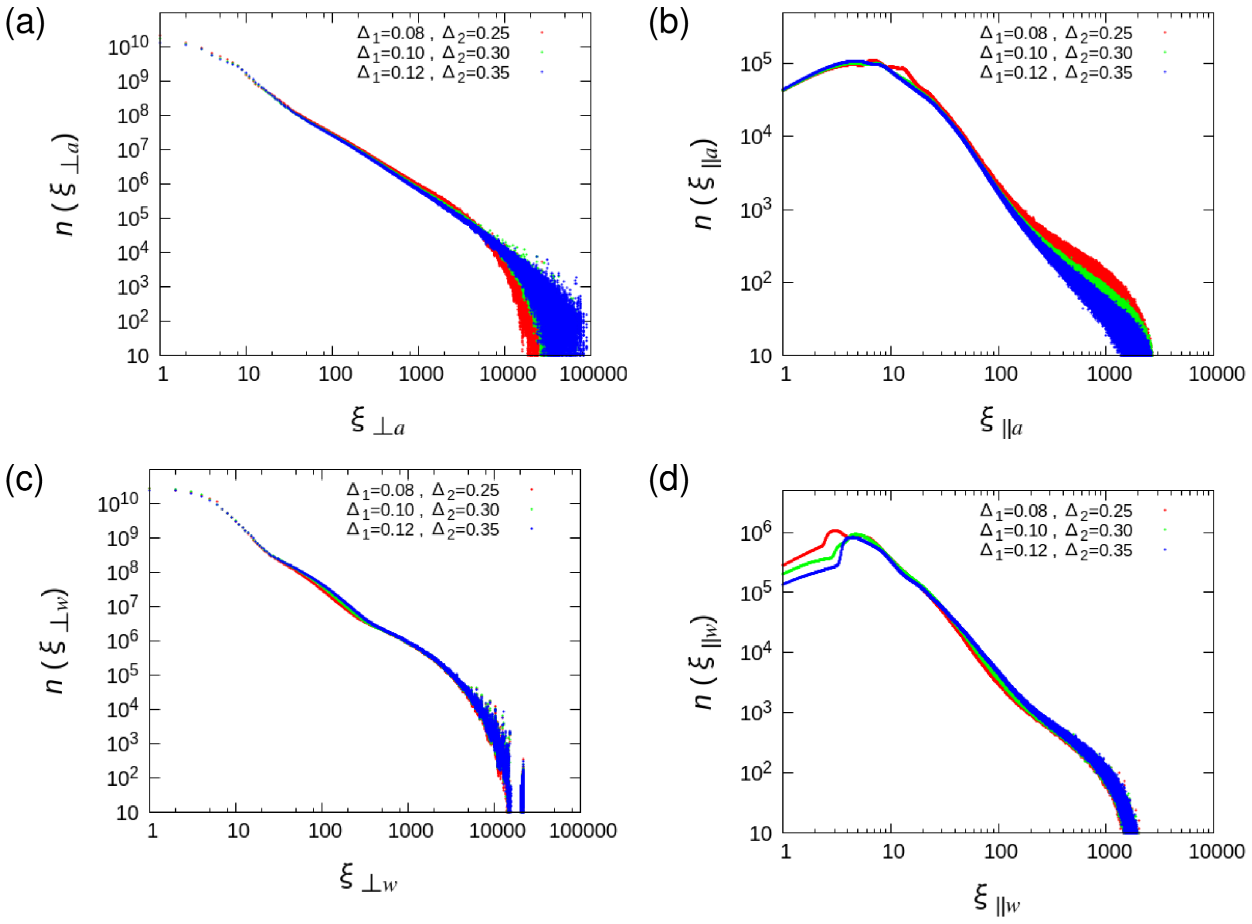


Figure S4: Histograms of the spatio-temporal gaps for different sets of $(\Delta_1, \Delta_2)$ as shown in the text. (a) Spatial gap $\xi_{\perp a}$ and (b) temporal gap $\xi_{\| a}$ between asynchronous sites. (c) Spatial gap $\xi_{\perp w}$ and (d) temporal gap $\xi_{\| w}$ between traveling wave sites.

## 2 Spatio-temporal correlation functions

The difference between the asynchronous and traveling wave states are seen by the spatio-temporal correlation functions $Q_a(x,t)$ and $Q_w(x,t)$. In Fig.2 of the main paper, we showed their cross sections at different time $t$. In Fig.S5, we plot their spatio-temporal profiles by colormaps. The statistics are taken on the same conditions as in Fig.2, i.e., with the phase delay $\alpha = 0.44$, system size $N = 131072$, and time window $250 < t < 1000$. The correlation function of the traveling wave state $Q_w(x,t)$ in Fig.S5(a) has a sharp peak propagating over a long distance with the velocity $v_w \simeq 2$. In contrast, the correlation function of the asynchronous state $Q_a(x,t)$ in Fig.S5(b) has only a short-ranged correlation both in space and time.

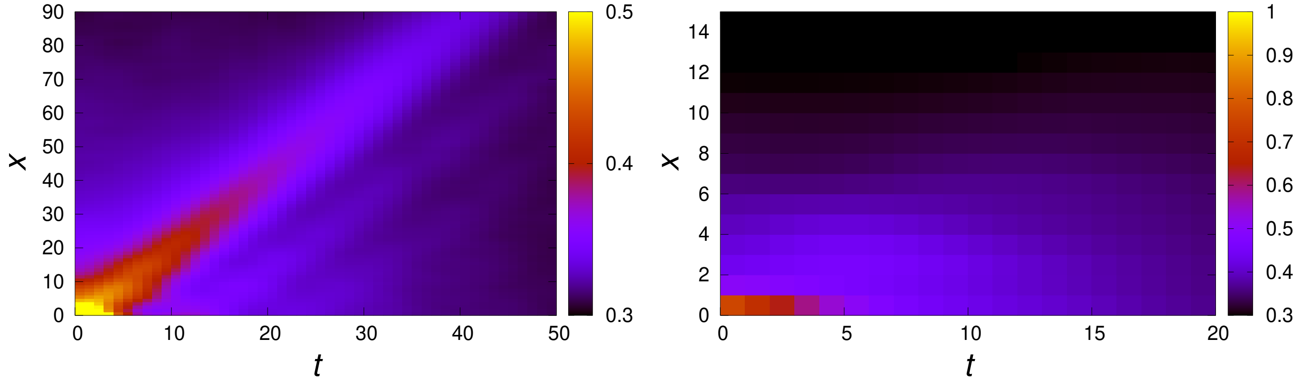


Figure S5: Spatio-temporal maps of the correlation functions for the (a) traveling wave state $Q_w(x,t)$, and (b) asynchronous state $Q_a(x,t)$.

## 3 Spatial fraction of the traveling waves sites

In Fig.S6, we show the time evolution of the fraction of traveling wave sites $\rho_w(t)$ for an $N = 131072$ system. At the critical point $\alpha = \alpha_c = 0.439$, the fraction shows initial growth until $t \simeq 200$ and then decreases rapidly until $t \simeq 5000$, before finally vanishing at $t \simeq 5 \times 10^5$. It decays to zero faster for smaller $\alpha$, while it converges to a finite value for $\alpha > \alpha_c$. For $\alpha = 0.447$, the fraction monotonically increases and converges to $\rho_w \simeq 0.4$.

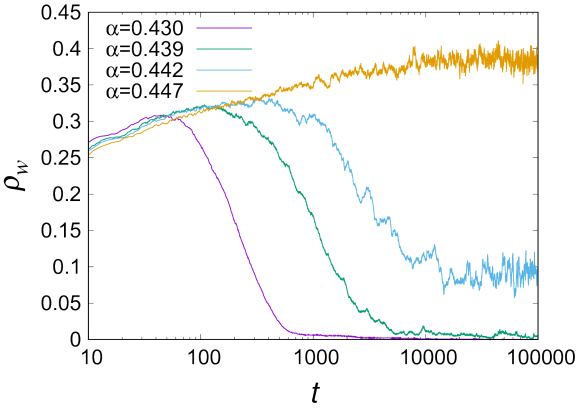


Figure S6: Time evolution of the fraction of traveling wave sites $\rho_w(t)$.

## 4 Spatio-temporal gaps between traveling waves sites

The histograms of the spatio-temporal gaps between traveling waves sites, which are already presented in Fig.S4 for discussion of the $\Delta_1$-dependence, are again shown in Fig.S7 for the standard parameters $\Delta_1 = 0.10, \Delta_2 = 0.30$. Statistics are taken with an $N = 16777216$ system and in the time window $0 < t < 3000$ as in the case of asynchronous sites. Both the spatial gap $\xi_{\perp w}$ and

temporal gap $\xi_{\parallel w}$ obey the power law distributions

$$n(\xi_{\perp w}) \sim \xi_{\perp w}^{-\mu_{\perp w}}, \quad n(\xi_{\parallel w}) \sim \xi_{\parallel w}^{-\mu_{\parallel w}}. \tag{4}$$

with the exponents

$$\mu_{\perp w} = 1.60 \pm 0.01, \quad \mu_{\parallel w} = 1.67 \pm 0.01. \tag{5}$$

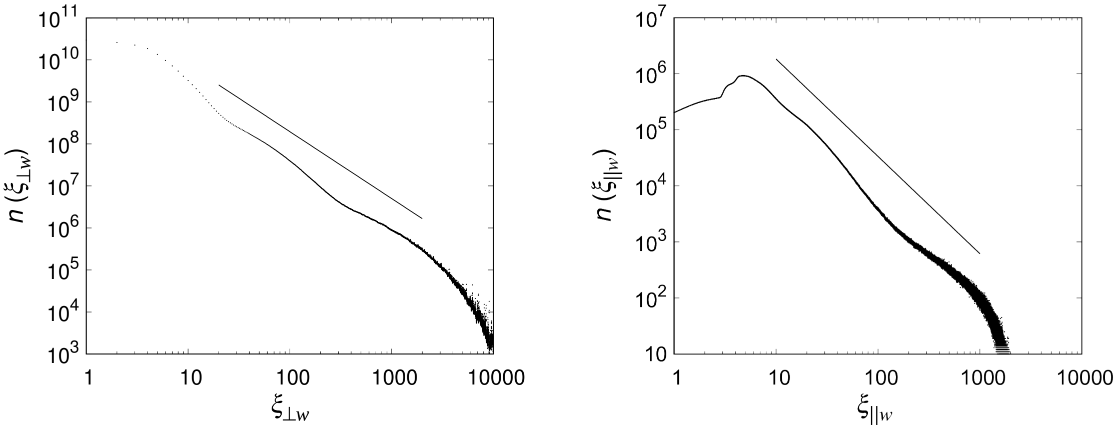


Figure S7: Histograms of the (a) spatial gap $\xi_{\perp w}$ and (b) temporal gap $\xi_{\parallel w}$ between traveling wave sites. Solid lines show the power-law fitting with the exponents $\mu_{\perp w} = 1.60$ and $\mu_{\parallel w} = 1.67$, respectively.

# 5 Rejuvenation of asynchronous sites

The definition of a rejuvenated site consists of the following conditions: (i) the site $x$ is asynchronous at time $t$: $\sigma_{x,t} = a$, (ii) the site and its nearest neighbors were not asynchronous at time $t-1$: $a \notin \{\sigma_{x+k,t-1}\}_{|k|\leq 1}$, and (iii) there were oppositely moving traveling waves within the third nearest neighbors at time $t-1$ : $w_+, w_- \in \{\sigma_{x+k,t-1}\}_{|k|\leq 3}$. Here we define the state value $\sigma_{x,t} = w_+$ ($w_-$) for a site occupied by a traveling wave moving in the + (−) directions, respectively. Because traveling waves move with a typical speed $v_w \simeq 2$, the condition (iii) is sufficient to pick up collision events. Also, the distance that asynchronous sites move in unit time is typically less than 1, as seen from Fig. S4. Therefore, the condition (ii) efficiently excludes the possibility that the asynchronous site at $(x, t)$ is continued from the previous time. In Fig.S8(a), we illustrate the definition by an example. In Fig.S8(b), we show the spatio-temporal map of asynchronous sites that are rejuvenated by collision of traveling waves. It shows that the traveling waves mediate non-local interactions between asynchronous sites and generate new asynchronous sites, which leads to a slower decay of the asynchronous fraction compared to the active fraction in DP.

# 6 Critical behaviors for the coupling range $L = 10$

In order to check the dependence on the coupling range $L$, we look at the critical behavior of the asynchronous fraction $\rho_a$ for $L = 10$. The system size $N = 131072$ is the same as in the case $L = 5$.

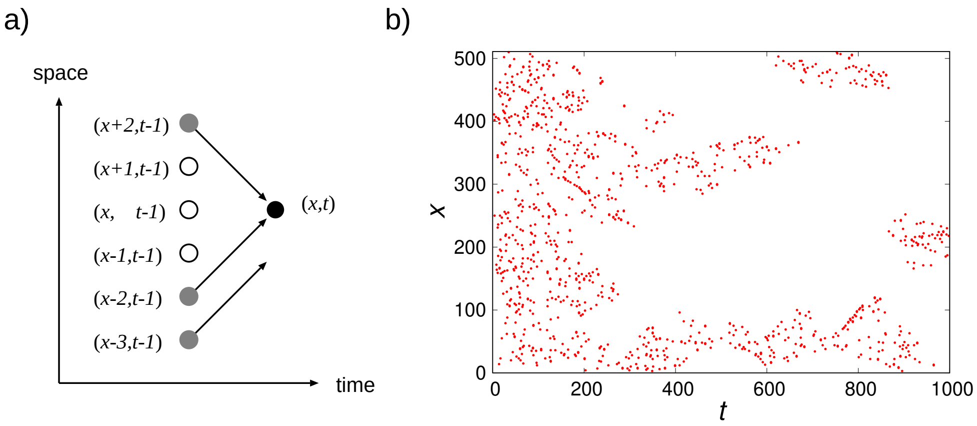


Figure S8: (a) Detection of rejuvenation of asynchronous sites by collision of traveling waves. The black circle shows an asynchronous site at $(x, t)$, and gray circles show traveling wave sites at time $t-1$ and within distance $\Delta x = 3$. White circles show synchronous sites. (b) Spatio-temporal map of the rejuvenated asynchronous sites.

The asynchronous fraction decay to zero for $\alpha \leq \alpha_c = 0.445$. The critical point is shifted upward by the increase of $L$. In Fig. S9, we show the dependence of $\rho_\alpha$ on $\alpha - \alpha_c$. The data are fitted by the power-law $\rho_a \sim (\alpha - \alpha_c)^{\beta_a}$, with the exponent $\beta_a = 1.73 \pm 0.17$. The exponent is smaller than the $L = 5$ case, indicating that the model exhibits a non-universal (parameter-dependent) critical behavior.

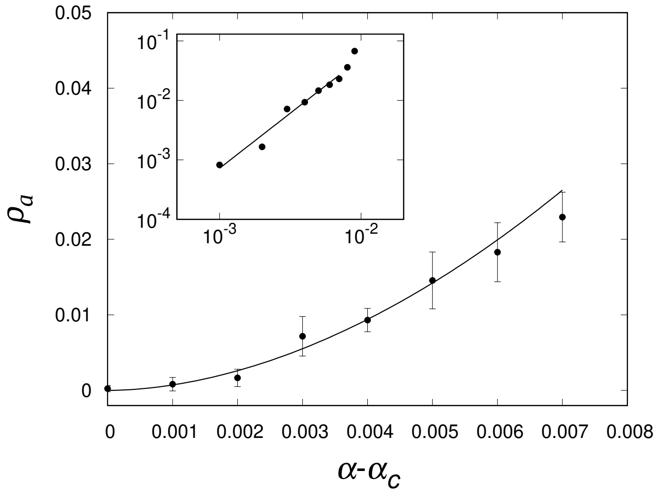


Figure S9: The steady state fraction of asynchronous sites $\rho_a$ versus $\alpha - \alpha_c$ for the coupling range $L = 10$. The critical point is $\alpha_c = 0.445$. Inset: logarithmic plot. Solid lines show the power law fitting with the exponent $\beta_a = 1.73$.
